# Supplementary material for: Fed-TGAN: Federated Learning Framework for Synthesizing Tabular Data
Source: arXiv:2108.07927 source file (2025-08-11)
Supplement: Supplementary file 1 [file appendix.tex]

\pagebreak
\appendix
   
\section{User Manual ZZ: this is old}
\setcounter{figure}{0} 
\subsection{Introduction}

The software demo developed by us comprises of a synthetic tabular data generation pipeline. It was implemented using python 3.7.* along with the flask library to work as a web appslication on a local server. The application functionality and usage can be found listed under the \nameref{Fmarker} \& \nameref{Umarker} sections respectively. In addition, a video of the demo can be seen \href{https://drive.google.com/file/d/1VK6479YPnjg0zVbfdgJb2G4_7lz2CWp6/view}{\underline{here}}. 

\subsection{Functionality}
\label{Fmarker}

Our demo comprises of the following salient features:

\begin{enumerate}
    
    \item \textbf{Synthetic Data Generator: }Our software is a cross-platform application that sits on top of a python interpreter. Moreover, it is relatively lightweight and can be set-up easily using pip. 
    Our application is also robust against missing values and supports date-type formats. We believe these factors increases its usability in real-world scenarios.  
    
    \item \textbf{Synthetic Data Evaluator: }In addition to our generator, we also provide a detailed evaluation of the synthetic data. The report provides end users with visual plots comparing the real and synthetic distributions of individual columns as shown in sub-figures \ref{fig:workclass} \& \ref{fig:age}  of Fig.~\ref{fig:visual_plots}.  In addition, the synthetic data's utility for ML applications along with its privacy preservability metrics are reported as can be seen in sub-figures \ref{fig:utility} \& \ref{fig:privacy} of Fig.~\ref{fig:efficacy}. Note that the table-evaluator\footnote{\url{ttps://github.com/Baukebrenninkmeijer/Table-Evaluator}} library aided us in generating this evaluating report.

\end{enumerate}

\subsection{Usage}
\label{Umarker}

The following step-by-step instructions are provided to allow end-users to use our product in a hassle-free manner. 

\begin{enumerate}[start=1,label={\bfseries Step \arabic*:},leftmargin=1.425cm]
    \item Open the terminal and navigate to the root directory of the software package to run the following command \texttt{python3 / python server.py}. 
    \item  \begin{minipage}[t]{\linewidth}
          \raggedright
          \adjustbox{valign=t}{%
            \includegraphics[width=.8\linewidth]{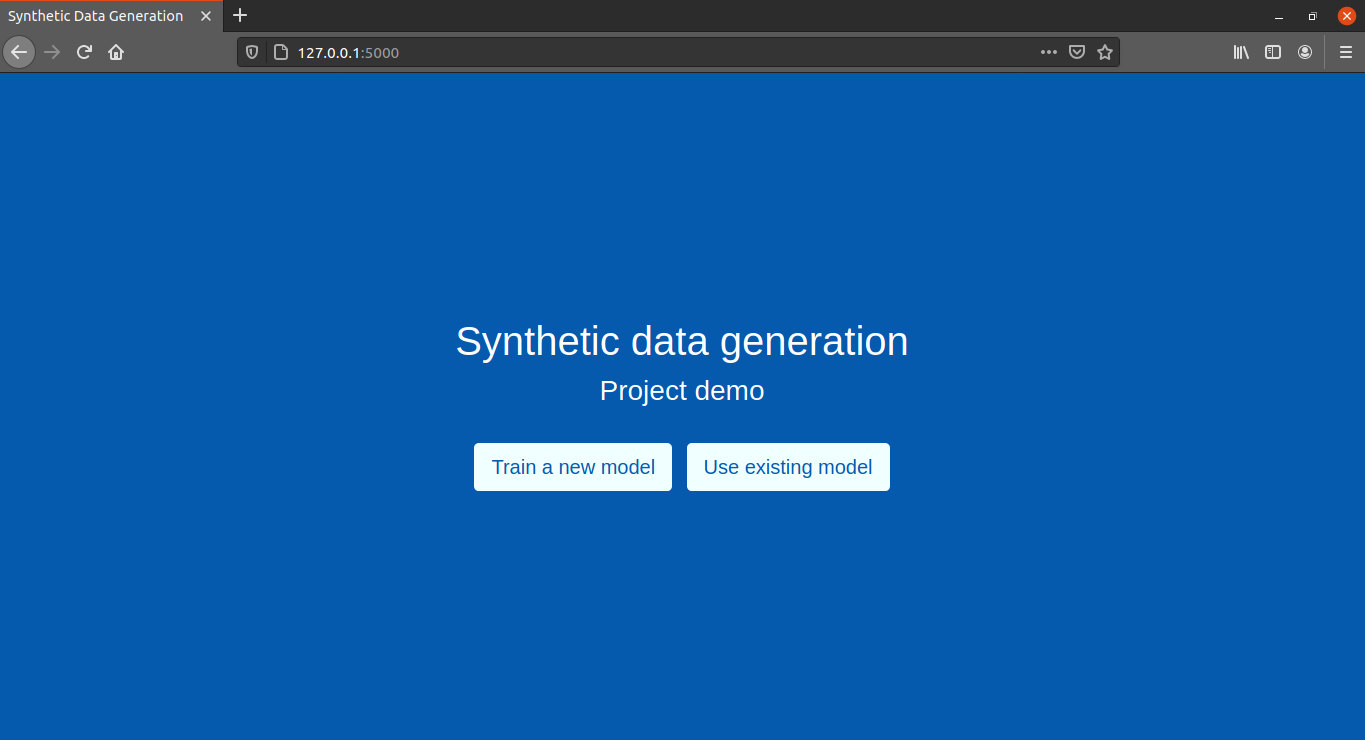}%
          }
          \medskip
          
          Open the browser, the application should now be available at the following address: \texttt{http://127.0.0.1:5000/}.

    \end{minipage}
    
    \item If this is the first time running the web application, it is advised to click on the ``Train a new model'' button to begin training the model with a dataset. Otherwise, click on the ``Use existing mode'' button to use an existing trained model.
    If you clicked on the ``Use existing mode'' button, please go to \textbf{step 8}. If not, please continue with the next step.
    
    \item \begin{minipage}[t]{\linewidth}
          \raggedright
          \adjustbox{valign=t}{%
            \includegraphics[width=.8\linewidth]{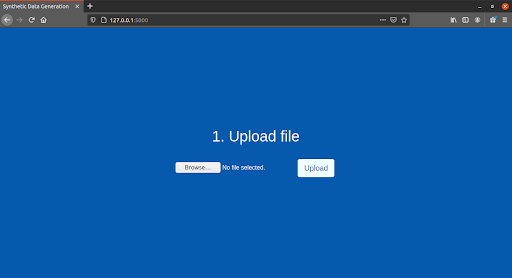}%
          }
          \medskip
    
     Click on the ``Browse'' button to select the dataset for which the model needs to train. Afterwards click on the ``Uploap'' button. 
     
    \end{minipage}

    \item \begin{minipage}[t]{\linewidth}
          \raggedright
          \adjustbox{valign=t}{%
            \includegraphics[width=.8\linewidth]{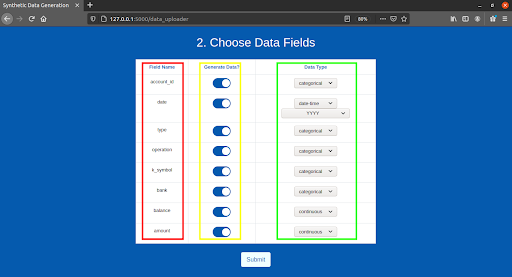}%
          }
          \medskip
    
     The software will auto-detect the column types, and will give the option to adjust a column's data type and inclusion in the training. Note that the red highlighted column shows the current columns in the uploaded \texttt{csv} file. The yellow highlighted column gives the option to include or exclude a particular column in the training process by clicking on the switch button. The highlighted green column is the auto detected data type. It also has the option to be adjusted as needed. Simply click on it and select the desired data type from the drop down menu. Click on the ``Submit'' button after choosing the right settings.
    \end{minipage}
    
    \item \begin{minipage}[t]{\linewidth}
          \raggedright
          \adjustbox{valign=t}{%
            \includegraphics[width=.8\linewidth]{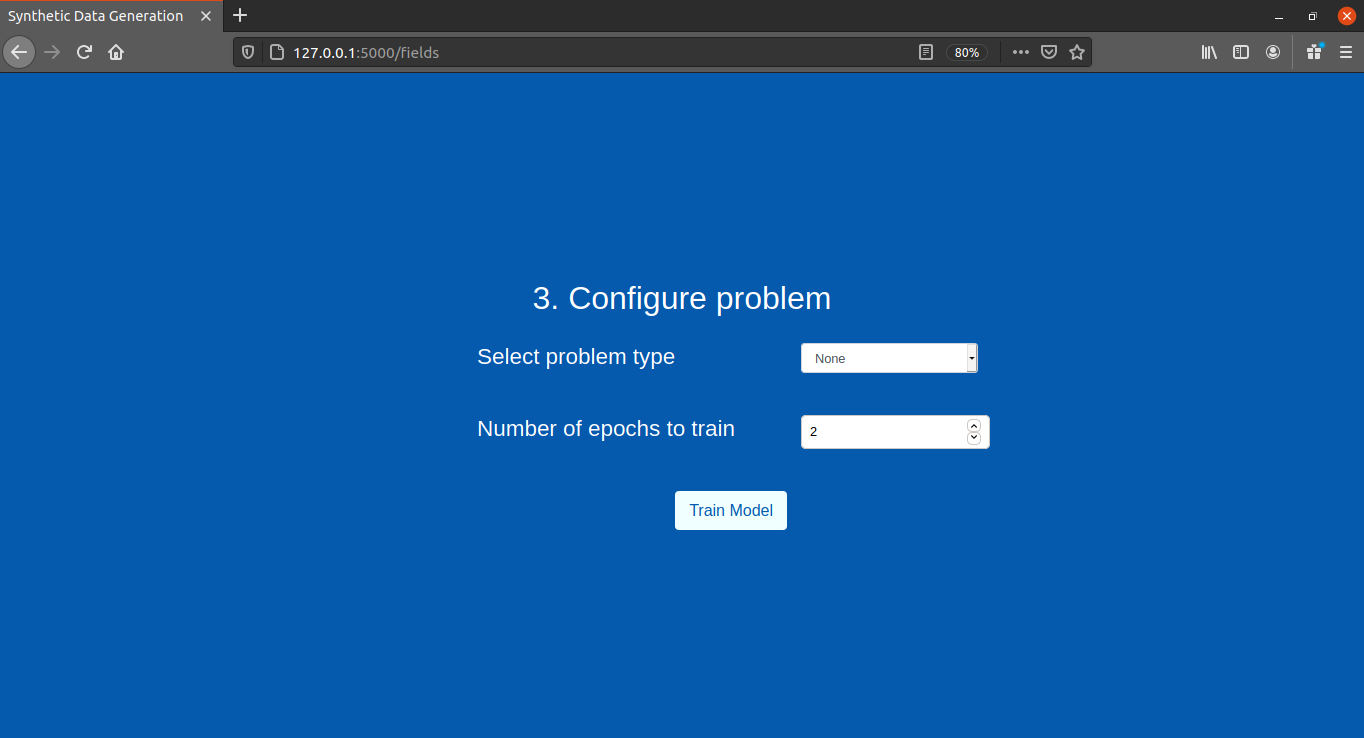}%
          }
          \medskip
    
     In the following page, specify the problem type for the given dataset. The software currently provides the following problem types: None, Binary Classification and Multi-class Classification. If unsure, leave it as None. Then enter the number of epochs needed to train the model. Click on ``Train Model'' to start the training. 

    \end{minipage}
    
    \item \begin{minipage}[t]{\linewidth}
          \raggedright
          \adjustbox{valign=t}{%
            \includegraphics[width=.8\linewidth]{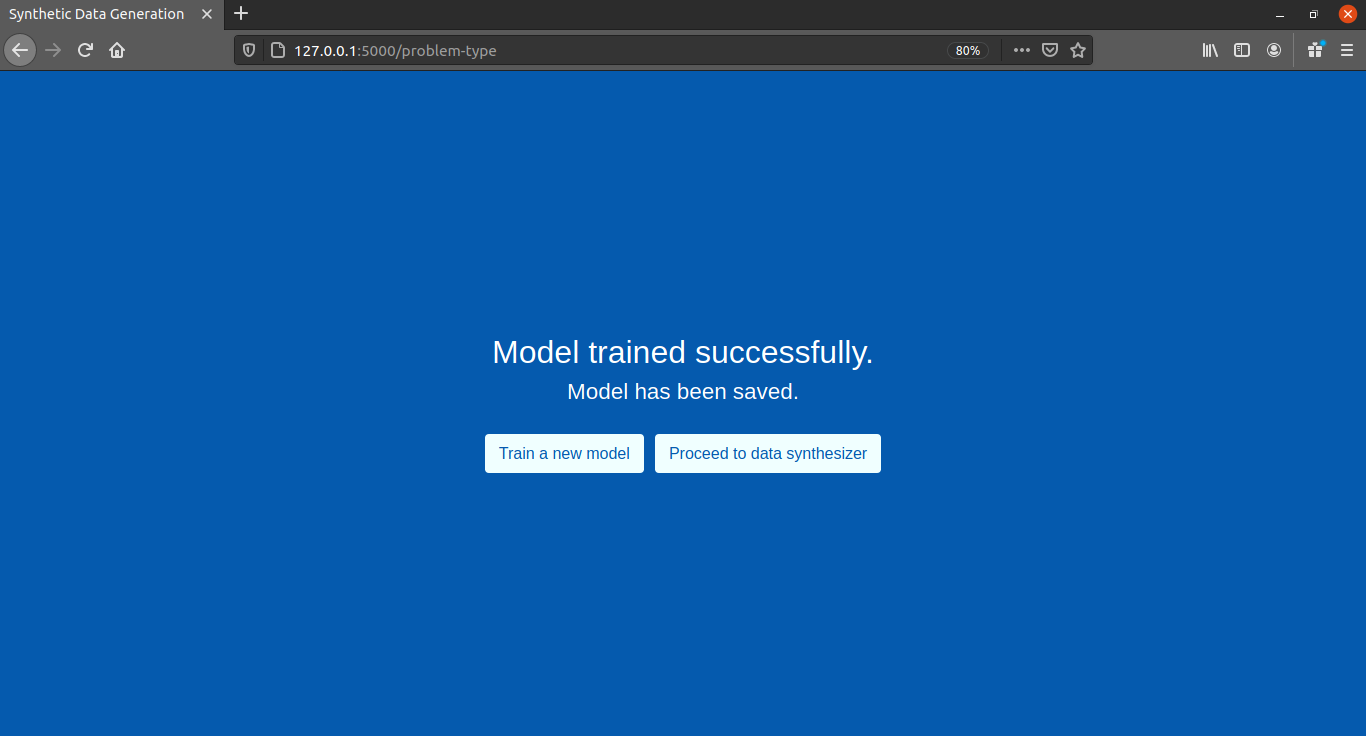}%
          }
          \medskip
    
     Once the model has finished training, the option to train a new model or proceed to the synthesizer is presented. To generate synthetic data, click on ``Proceed to data synthesizer''.

    \end{minipage}
    
    \item \begin{minipage}[t]{\linewidth}
          \raggedright
          \adjustbox{valign=t}{%
            \includegraphics[width=.8\linewidth]{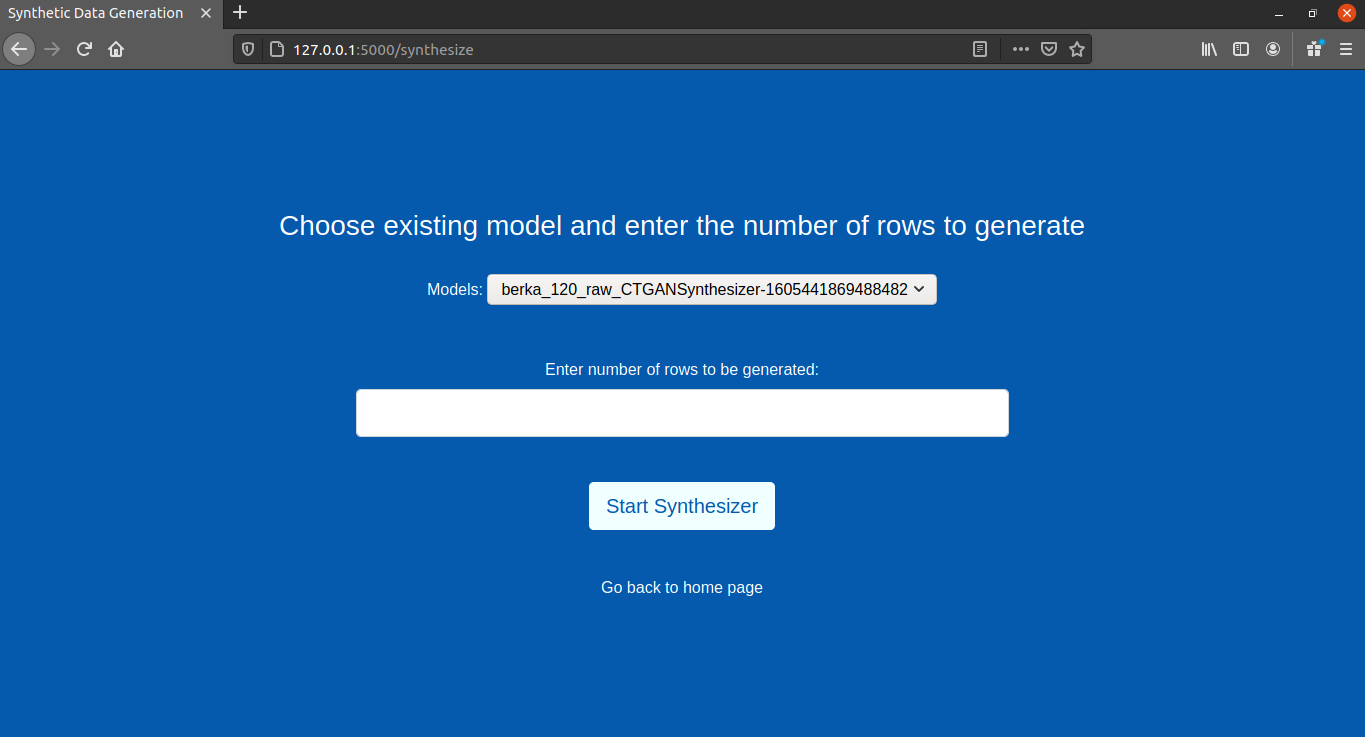}%
          }
          \medskip
    
     The trained models can be found in the dropdown menu of the Models field, as seen in the figure above. Click on it, and select the trained model. After this, type the amount of rows to be generated in the second field, and click on ``Start Synthesizer'' to start the process. 

    \end{minipage}
    
    \item \begin{minipage}[t]{\linewidth}
          \raggedright
          \adjustbox{valign=t}{%
            \includegraphics[width=.8\linewidth]{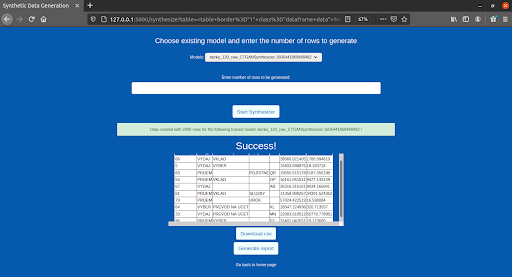}%
          }
          \medskip
    
     Once the data is generated, the following page shows a snippet of the synthetic data. The generated data can be saved locally by clicking on ``Download csv''. This page also gives you the option to generate a report for the given data. In order to generate the report in PDF format, simply click on ``Generate report'' and continue with step 10. 

    \end{minipage}
    
    \item \begin{minipage}[t]{\linewidth}
          \raggedright
          \adjustbox{valign=t}{%
            \includegraphics[width=.8\linewidth]{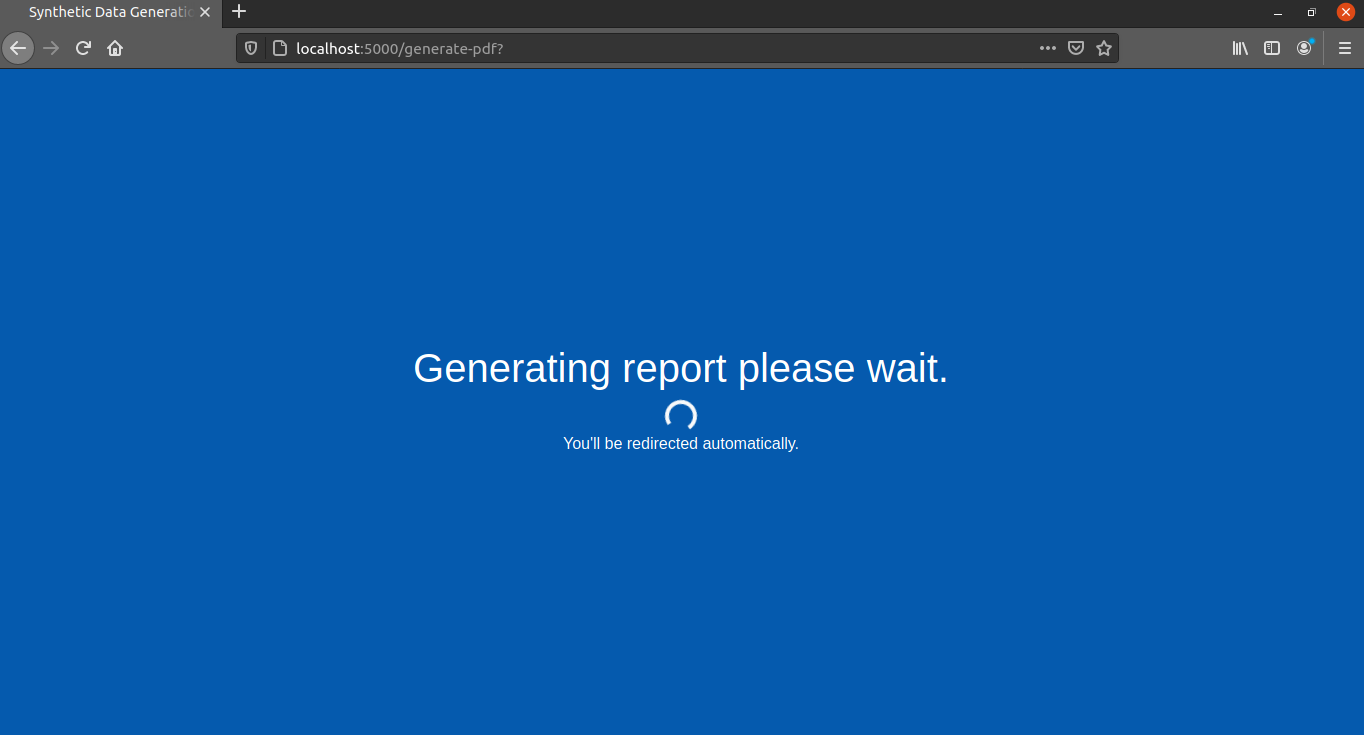}%
          }
          \medskip
    
    The following page is presented while the report is being generated. It will automatically redirect to the PDF once it is completed.
    \end{minipage}
    
    \item \begin{minipage}[t]{\linewidth}
          \raggedright
          \adjustbox{valign=t}{%
            \includegraphics[width=.8\linewidth]{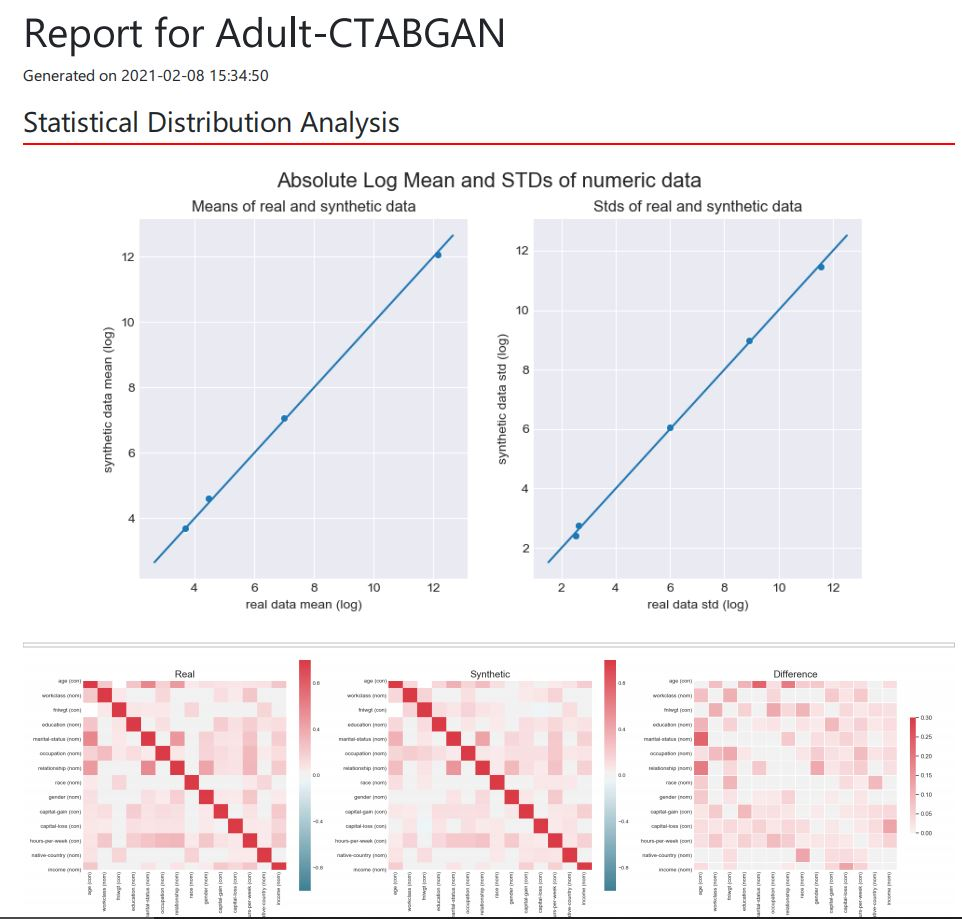}%
          }
          \medskip
    
    Finally, once the PDF has been generated, it can be saved locally by clicking on ``Save as'' or ``Print'' in the browser.  
    \end{minipage}

\end{enumerate}

\begin{figure}[H]
	\begin{center}
		\subfloat[Cumulative distribution comparison of Age in Adult]{
			\includegraphics[width=0.47\columnwidth,height=4.5cm]{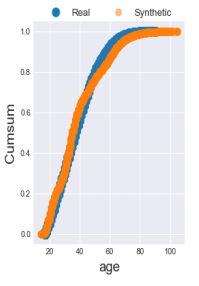}
		    \label{fig:workclass}
		}
		\hfil
		\subfloat[Frequency comparison of categories within Workclass in Adult]{
			\includegraphics[width=0.47\columnwidth,height=4.25cm]{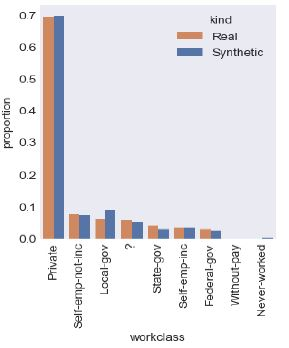}
			\label{fig:age}
		}
		\caption{Visual plots comparing the generated vs real data distribution.}
		\label{fig:visual_plots}
	\end{center}
\end{figure}

\begin{figure}[H]
	\begin{center}
		\subfloat[ML Utility]{
			\includegraphics[width=0.57\columnwidth]{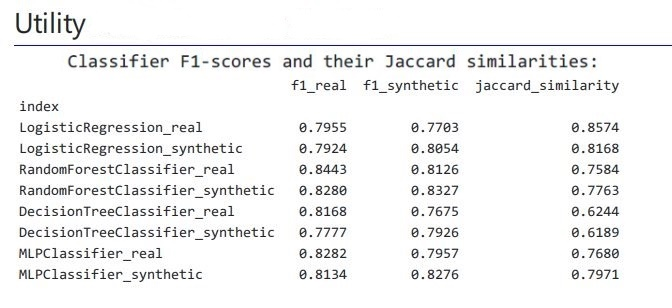}
		    \label{fig:utility}
		}
		\hfil
		\subfloat[Privacy Preservability]{
			\includegraphics[width=0.57\columnwidth]{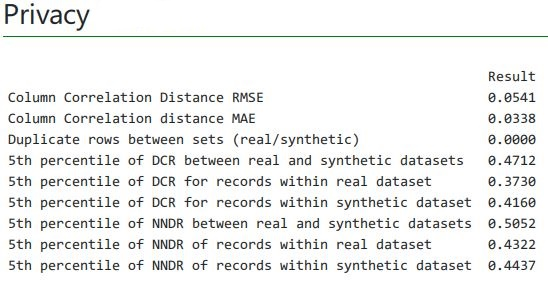}
			\label{fig:privacy}
		}
		\caption{ML utility and privacy preservability of the generated data.}
		\label{fig:efficacy}
	\end{center}
\end{figure}
